# Supplementary material for: CLIP-UP: A Simple and Efficient Mixture-of-Experts CLIP Training Recipe with Sparse Upcycling
Source: arXiv:2502.00965 source file (2025-05-25)
Supplement: Supplementary file 1 [file appendix_capacity_factor.tex]

\begin{table*}[h]
\caption{All results from Figure \ref{fig:capacity-compare}}
\label{tab:appendix-capacity-compare}
\vskip 0.15in
\begin{center}
\begin{small}
\begin{sc}
\begin{tabular}{lccccc}
\toprule
\multirow{3}{*}{Model} &\multicolumn{1}{c}{Imagenet} &\multicolumn{2}{c}{COCO} &\multicolumn{2}{c}{Flickr30K} \\
&Accuracy@1 &T2I R@1 &I2T R@1 &T2I R@1 &I2T R@1 \\

\midrule
% \rowcolor{lightgray} 
$C_{image}=2, C_{text}=2$ & 76.9 &52.1 &71.5 &80.9 &92.3 \rule{0pt}{3ex} \\
% \quad+LIMOE Aux. Loss &73.1 &49.7 &69.7 &75.6 &87.9 \rule{0pt}{3ex} \\
% \quad $\Delta$ & +3.4 & +3.0 & +4.1 & +4.2 & +1.6 \\
% \cdashline{1-6}
% \rowcolor{lightgray} 
$C_{image}=4, C_{text}=2$ &78.4 &46.3 &66.9 &75.5 &90.2 \rule{0pt}{3ex} \\
% \quad+LIMOE Aux. Loss &73.9 &50.9 &70.1 &73.8 &85.5 \rule{0pt}{3ex} \\
% \quad $\Delta$ & -1.3 & -0.7 & -2.6 & -4.2 & -6.5 \\
% \cdashline{1-6}
% \rowcolor{lightgray} 
% Separated &74.5 &\textbf{53.1} &70.6 &78.3 &88.2 \rule{0pt}{3ex} \\
% % \quad+LIMOE Aux. Loss &72.6 &46.4 &62.6 &73.4 &85.2 \rule{0pt}{3ex} \\
% % \quad $\Delta$ & -2.0 & -6.7 & -8.0 & -4.9 & -3.0 \\
% % \cdashline{1-6}
% % \rowcolor{lightgray} 
% Separated-Up &\textbf{76.9} &52.1 &71.5 &\textbf{80.9} &\textbf{92.3} \rule{0pt}{3ex} \\
% \quad+LIMOE Aux. Loss &75.9 &52.9 &73.5 &81.3 &92.5 \rule{0pt}{3ex} \\
% \quad $\Delta$ & -1.0 & +0.8 & +2.0 & +0.4 & +0.2 \\
\bottomrule
\end{tabular}
\end{sc}
\end{small}
\end{center}
\end{table*}
